# Supplementary material for: On the Generation of Electronic Ring Currents under Vibronic Coupling Effects
Source: arXiv:2010.02308 source file (2020-10-05)
Supplement: Supplementary file 1 [file EcurrentsJCP_SI.pdf]

**Supporting Information for the 'On the Generation of Electronic Ring Currents under Vibronic Coupling Effects'**

Krishna Reddy Nandipati[1, a)] and Oriol Vendrell[1, 2, b)]

[1)] *Theoretische Chemie, Physikalisch-Chemisches Institut, Universität Heidelberg, Im Neuneheimer Feld 229, 69120 Heidelberg, Germany*

[2)] *Centre for Advanced Materials, Universität Heidelberg, Im Neuenheimer Feld 205, 69120 Heidelberg, Germany*

[a)]e-mail: krishna.nandipati@pci.uni-heidelberg.de

[b)]e-mail: oriol.vendrell@pci.uni-heidelberg.de

**General expression for the current for a superposition of vibronic states:**

The general form of laser-driven vibronic wavepacket $|\psi(t)\rangle$ is given as

$$|\psi(t)\rangle = A_0(t)|0_0\rangle + \sum_{q>0}\sum_{j_q}\Big(A_{j_q}(t)|j_q\rangle + A_{j_{-q}}(t)|j_{-q}\rangle\Big) \tag{S1}$$

By projecting $|\psi(t)\rangle$ on to the electronic $l$ basis and using $P_l(t) = |\langle l|\psi(t)\rangle|^2$ in Eq. (11) in the main text, we get

$$J_e(t) = \frac{\hbar}{4\pi^2 I_\theta}\sum_{l>0} l\Big(\langle\psi(t)|l\rangle\langle l|\psi(t)\rangle - \langle\psi(t)|-l\rangle\langle -l|\psi(t)\rangle\Big). \tag{S2}$$

Using the Born-Huang expansion of the vibronic eigenstates $j_{\pm q}$ [cf. Eq. (14) in the main text] in Eq. (S1), the $\langle l|\psi(t)\rangle$ is given by

$$\langle l|\psi(t)\rangle = \sum_{q>0}\sum_{j_q}\Big[A_{j_q}(t)c^{j_q}_{q-l,l}|k=q-l\rangle + A_{j_{-q}}(t)c^{j_{-q}}_{-q-l,l}|k=-q-l\rangle\Big], \tag{S3}$$

here the index $k$ is necessarily different for all $q^{'}s$, within a given $l$. Thus it follows that

$$\langle\psi(t)|l\rangle\langle l|\psi(t)\rangle = \sum_{q>0}\sum_{j_q j'_q}\Big(A^*_{j_q}(t)A_{j'_q}(t)c^{j^*_q}_{q-l,l}c^{j'_q}_{q-l,l} + A^*_{j_{-q}}(t)A_{j'_{-q}}(t)c^{j^*_{-q}}_{-q-l,l}c^{j'_{-q}}_{-q-l,l}\Big), \tag{S4}$$

replacing $l$ by -$l$ in Eq. (S5) we get the corresponding expression for $\langle\psi(t)|-l\rangle\langle -l|\psi(t)\rangle$. Now the term in the parenthesis of Eq. (S2) can be written as

$$\langle\psi(t)|l\rangle\langle l|\psi(t)\rangle = \sum_{q>0}\sum_{j_q j'_q}\Big(A^*_{j_q}(t)A_{j'_q}(t)c^{j^*_q}_{q-l,l}c^{j'_q}_{q-l,l} + A^*_{j_{-q}}(t)A_{j'_{-q}}(t)c^{j^*_{-q}}_{-q-l,l}c^{j'_{-q}}_{-q-l,l}\Big), \tag{S5}$$

$$\begin{aligned}
\langle\psi(t)|l\rangle\langle l|\psi(t)\rangle - \langle\psi(t)|-l\rangle\langle -l|\psi(t)\rangle &= \sum_{q>0}\sum_{j_q j'_q}\Bigg[\Big(A^*_{j_q}(t)A_{j'_q}(t)c^{j^*_q}_{q-l,l}c^{j'_q}_{q-l,l} + A^*_{j_{-q}}(t)A_{j'_{-q}}(t)c^{j^*_{-q}}_{-q-l,l}c^{j'_{-q}}_{-q-l,l}\Big) \\
&\quad - \Big(A^*_{j_q}(t)A_{j'_q}(t)c^{j^*_q}_{q+l,-l}c^{j'_q}_{q+l,-l} + A^*_{j_{-q}}(t)A_{j'_{-q}}(t)c^{j^*_{-q}}_{-q+l,-l}c^{j'_{-q}}_{-q+l,-l}\Big)\Bigg] \\
&= \sum_{q>0}\sum_{j_q j'_q}\Big(A^*_{j_q}(t)A_{j'_q}(t)Y^{(l)}_{j_q j'_q} + A^*_{j_{-q}}(t)A_{j'_{-q}}(t)Y^{(l)}_{j_{-q}j'_{-q}}\Big) \\
&= \sum_{q>0}\sum_{j_q j'_q}\Big(A^*_{j_q}(t)A_{j'_q}(t) - A^*_{j_{-q}}(t)A_{j'_{-q}}(t)\Big)Y^{(l)}_{j_q j'_q}
\end{aligned} \tag{S6}$$

where $Y^{(l)}_{j_{\pm q} j'_{\pm q}} = c^{j^*_{\pm q}}_{\pm q-l,l} c^{j'_{\pm q}}_{\pm q-l,l} - c^{j^*_{\pm q}}_{\pm q+l,-l} c^{j'_{\pm q}}_{\pm q+l,-l}$ and we have used the relations $c^{j_q}_{q-l,l} = c^{j_{-q}}_{-q+l,-l}$; $c^{j'_q}_{q-l,l} = c^{j'_{-q}}_{-q+l,-l}$ (same goes for complex conjugates of the coefficients) which imply $Y_{j_q j'_q} = -Y_{j_{-q} j'_{-q}}$ in the above.

Substituting Eq. (S6) into Eq. (S2) and adding the terms contributed by the individual triads of $j_q$ and the $j_{-q}$, we get the general expression for the current:

$$
\begin{aligned}
J_e(t) = \frac{\hbar}{4\pi^2 I_\theta}\Bigg[\sum_{l>0} l\Bigg[\sum_{q>0}\Bigg\{\sum_{j_q}\Big(|A_{j_q}(t)|^2 - |A_{j_{-q}}|^2\Big)Y^{(l)}_{j_q} \\
+\sum_{j_q}\sum_{j'_q<j_q}\Big(2\Re\{A^*_{j_q}(t)A_{j'_q}(t)\} - 2\Re\{A^*_{j_{-q}}(t)A_{j'_{-q}}(t)\}\Big)Y^{(l)}_{j_q j'_q}\Bigg\}\Bigg]\Bigg].
\end{aligned} \tag{S7}
$$

The final expression has one diagonal contribution per eigenstate of the $q$-th with a contribution to electronic angular momentum $l$. The off-diagonal contribution corresponds to the coherent contribution of eigenstates within the $q$-th to the $l$-th angular momentum. Note in the second line that quantum coherence is limitted to eigenstates within each block $q$ and $-q$ but not across blocks.
